# Supplementary material for: The Reduction of Magnetic Reconnection Outflow Jets to Sub-Alfv\'enic Speeds
Source: arXiv:1804.09805 source file (2018-04-25)
Supplement: Supplementary file 1 [file sup_mat.pdf]

# The Reduction of Magnetic Reconnection Outflow Jets to Sub-Alfvénic Speeds: Supplementary Material

Colby C. Haggerty\*

*Department of Astronomy and Astrophysics, University of Chicago, Chicago, IL 60637, USA and  
Bartol Research Institute, Department of Physics and Astronomy,  
University of Delaware, Newark, DE 19716, USA*

Michael A. Shay and Alexandros Chasapis

*Bartol Research Institute, Department of Physics and Astronomy,  
University of Delaware, Newark, DE 19716, USA*

Tai D. Phan

*Space Sciences Laboratory, University of California, Berkeley, California 94720, USA*

James F. Drake

*Institute for Research in Electronics and Applied Physics,  
University of Maryland, College Park, Maryland 20742, USA*

Kittipat Malakit

*Department of Physics, Faculty of Science and Technology,  
Thammasat University, Pathum Thani, Thailand*

Paul A. Cassak

*Department of Physics and Astronomy, West Virginia University, Morgantown, West Virginia 26506, USA*

Rungployphan Kieokaew

*CGAFD, Mathematics, CEMPS, University of Exeter, Exeter, UK*

(Dated: April 20, 2018)

## SIMULATIONS

Bellow we present the the initial parameters of the 81 different PIC simulations used in this study where  $m_i/m_e$  is the artificial ion to electron mass ratio,  $B_r$  is the magnitude of the reconnection component of the upstream magnetic field,  $B_g$  the upstream component of the magnetic field normal to the current sheet and the outflow

direction called the guide field,  $n_{in}$  the initial upstream density,  $T_e$  and  $T_i$  the initial electron and ion temperature respectively and  $\beta_r$  the total plasma beta based on the reconnecting component of the magnetic field.

---

\* CHaggerty@UChicago.edu

| Run    | $m_i/m_e$ | $B_r$ | $B_g$ | $n_{in}$ | $T_e$  | $T_i$  | $\beta_r$ |
|--------|-----------|-------|-------|----------|--------|--------|-----------|
| 14     | 25.0      | 1.0   | 0.0   | 0.04     | 0.25   | 2.25   | 0.20      |
| 15     | 25.0      | 1.0   | 0.0   | 0.04     | 1.0    | 9.0    | 0.80      |
| 16     | 25.0      | 1.0   | 0.0   | 0.04     | 1.8    | 9.0    | 0.86      |
| 17     | 25.0      | 1.0   | 0.0   | 0.04     | 9.0    | 9.0    | 1.44      |
| 20     | 25.0      | 1.0   | 0.0   | 0.2      | 22.5   | 2.5    | 10.0      |
| 301    | 25.0      | 1.0   | 0.0   | 0.2      | 0.25   | 0.25   | 0.20      |
| 302    | 25.0      | 1.0   | 1.0   | 0.2      | 0.25   | 0.25   | 0.20      |
| 303    | 25.0      | 1.0   | 0.0   | 0.2      | 2.25   | 0.25   | 1.00      |
| 304    | 25.0      | 1.0   | 1.0   | 0.2      | 2.25   | 0.25   | 1.00      |
| 305    | 25.0      | 1.0   | 0.0   | 0.2      | 0.25   | 2.25   | 1.00      |
| 306    | 25.0      | 1.0   | 1.0   | 0.2      | 0.25   | 2.25   | 1.00      |
| 307    | 25.0      | 1.0   | 0.0   | 1.0      | 0.25   | 0.25   | 1.00      |
| 309    | 25.0      | 1.0   | 0.0   | 0.04     | 2.25   | 0.25   | 0.20      |
| 310001 | 25.0      | 2.236 | 0.0   | 0.2      | 2.25   | 0.25   | 0.20      |
| 312001 | 25.0      | 0.447 | 0.447 | 0.2      | 0.25   | 0.25   | 1.00      |
| 313    | 25.0      | 1.0   | 1.0   | 0.04     | 2.25   | 0.25   | 0.20      |
| 314001 | 25.0      | 2.236 | 2.236 | 0.2      | 2.25   | 0.25   | 0.20      |
| 318001 | 25.0      | 2.236 | 2.236 | 0.2      | 0.25   | 2.25   | 0.20      |
| 319    | 25.0      | 0.447 | 0.0   | 0.2      | 2.25   | 0.25   | 5.00      |
| 320    | 25.0      | 0.447 | 0.447 | 0.2      | 2.25   | 0.25   | 5.00      |
| 323    | 25.0      | 1.0   | 0.0   | 0.2      | 1.25   | 0.25   | 0.60      |
| 324    | 25.0      | 1.0   | 1.0   | 0.2      | 1.25   | 0.25   | 0.60      |
| 325    | 25.0      | 1.0   | 0.0   | 0.2      | 0.3125 | 0.0625 | 0.15      |
| 326    | 25.0      | 1.0   | 1.0   | 0.2      | 0.3125 | 0.0625 | 0.15      |
| 327    | 25.0      | 1.0   | 0.0   | 0.2      | 5.0    | 1.0    | 2.40      |
| 328    | 25.0      | 1.0   | 1.0   | 0.2      | 5.0    | 1.0    | 2.40      |
| 601    | 25.0      | 1.0   | 0.0   | 0.2      | 1.25   | 0.25   | 0.60      |
| 602    | 25.0      | 0.447 | 0.0   | 0.2      | 1.25   | 0.25   | 3.00      |
| 603    | 25.0      | 2.236 | 0.0   | 0.2      | 1.25   | 0.25   | 0.12      |
| 604    | 25.0      | 1.0   | 1.0   | 0.2      | 1.25   | 0.25   | 0.60      |
| 621    | 25.0      | 1.0   | 0.0   | 0.2      | 1.25   | 0.25   | 0.60      |
| 622    | 25.0      | 0.447 | 0.0   | 0.2      | 1.25   | 0.25   | 3.00      |
| 623    | 25.0      | 2.236 | 0.0   | 0.2      | 1.25   | 0.25   | 0.12      |
| 624    | 25.0      | 1.0   | 1.0   | 0.2      | 1.25   | 0.25   | 0.60      |
| 625    | 25.0      | 0.447 | 0.447 | 0.2      | 1.25   | 0.25   | 3.00      |
| 626    | 25.0      | 2.236 | 2.236 | 0.2      | 1.25   | 0.25   | 0.12      |
| 629    | 25.0      | 0.75  | 1.0   | 0.2      | 1.25   | 0.25   | 1.07      |
| 632    | 25.0      | 1.0   | 0.5   | 0.2      | 1.25   | 0.25   | 0.60      |

| Run | $m_i/m_e$ | $B_r$    | $B_g$ | $n_{in}$ | $T_e$  | $T_i$  | $\beta_r$ |
|-----|-----------|----------|-------|----------|--------|--------|-----------|
| 633 | 25.0      | 1.0      | 0.75  | 0.2      | 1.25   | 0.25   | 0.60      |
| 634 | 25.0      | 1.0      | 0.083 | 0.2      | 1.25   | 0.25   | 0.60      |
| 635 | 25.0      | 1.0      | 0.167 | 0.2      | 1.25   | 0.25   | 0.60      |
| 641 | 25.0      | 1.0      | 0.0   | 0.2      | 1.0    | 1.0    | 0.80      |
| 642 | 25.0      | 1.0      | 0.25  | 0.2      | 1.0    | 1.0    | 0.80      |
| 644 | 25.0      | 1.0      | 0.75  | 0.2      | 1.0    | 1.0    | 0.80      |
| 645 | 25.0      | 1.0      | 1.0   | 0.2      | 1.0    | 1.0    | 0.80      |
| 646 | 25.0      | 1.0      | 0.08  | 0.2      | 1.0    | 1.0    | 0.80      |
| 647 | 25.0      | 1.0      | 0.17  | 0.2      | 1.0    | 1.0    | 0.80      |
| 651 | 25.0      | 2.24     | 0.0   | 0.2      | 6.25   | 1.25   | 0.60      |
| 652 | 25.0      | 0.45     | 0.0   | 0.2      | 0.25   | 0.05   | 0.59      |
| 655 | 25.0      | 1.0      | 0.0   | 0.04     | 6.25   | 1.25   | 0.60      |
| 657 | 25.0      | 0.45     | 0.0   | 0.04     | 1.25   | 0.25   | 0.59      |
| 661 | 25.0      | 1.673    | 0.0   | 0.2      | 3.5    | 0.7    | 0.60      |
| 662 | 25.0      | 0.74833  | 0.0   | 0.04     | 3.5    | 0.7    | 0.60      |
| 671 | 25.0      | 1.0      | 0.0   | 0.2      | 0.75   | 0.75   | 0.60      |
| 672 | 25.0      | 0.447    | 0.0   | 0.2      | 0.15   | 0.15   | 0.60      |
| 673 | 25.0      | 2.236    | 0.0   | 0.2      | 3.75   | 3.75   | 0.60      |
| 674 | 25.0      | 1.0      | 0.0   | 0.2      | 1.35   | 0.15   | 0.60      |
| 675 | 25.0      | 0.447    | 0.0   | 0.2      | 0.27   | 0.03   | 0.60      |
| 676 | 25.0      | 2.236    | 0.0   | 0.2      | 6.75   | 0.75   | 0.60      |
| 681 | 25.0      | 0.447    | 0.45  | 0.2      | 0.25   | 0.05   | 0.60      |
| 682 | 25.0      | 2.236    | 2.24  | 0.2      | 6.25   | 1.25   | 0.60      |
| 691 | 25.0      | 2.236    | 0.0   | 0.2      | 1.25   | 1.25   | 0.20      |
| 692 | 25.0      | 0.447    | 0.0   | 0.2      | 0.05   | 0.05   | 0.20      |
| 693 | 100.0     | 1.0      | 0.0   | 0.2      | 0.25   | 0.25   | 0.20      |
| 694 | 25.0      | 1.0      | 0.0   | 0.2      | 0.25   | 0.08   | 0.13      |
| 695 | 25.0      | 1.0      | 0.0   | 0.2      | 0.08   | 0.25   | 0.13      |
| 701 | 100.0     | 1.0      | 0.0   | 0.2      | 1.25   | 0.25   | 0.60      |
| 702 | 100.0     | 1.0      | 1.0   | 0.2      | 1.25   | 0.25   | 0.60      |
| 703 | 100.0     | 0.447    | 0.0   | 0.2      | 1.25   | 0.25   | 3.00      |
| 705 | 100.0     | 2.236    | 0.0   | 0.2      | 1.25   | 0.25   | 0.12      |
| 706 | 100.0     | 2.236    | 2.236 | 0.2      | 1.25   | 0.25   | 0.12      |
| 707 | 100.0     | 1.0      | 0.0   | 0.2      | 0.3125 | 0.0625 | 0.15      |
| 708 | 100.0     | 1.0      | 1.0   | 0.2      | 0.3125 | 0.0625 | 0.15      |
| 712 | 100.0     | 2.24     | 0.0   | 0.2      | 6.25   | 1.25   | 0.60      |
| 714 | 100.0     | 1.67     | 0.0   | 0.2      | 3.5    | 0.7    | 0.60      |
| 715 | 100.0     | 0.748331 | 0.0   | 0.04     | 3.5    | 0.7    | 0.60      |
| 804 | 400.0     | 1.0      | 0.0   | 0.2      | 1.25   | 0.25   | 0.60      |
| 901 | 25.0      | 2.236    | 0.0   | 0.2      | 0.25   | 2.25   | 0.20      |
| 904 | 100.0     | 2.236    | 0.0   | 0.2      | 0.25   | 2.25   | 0.20      |
| 930 | 25.0      | 1.0      | 0.0   | 0.04     | 0.45   | 2.25   | 0.22      |
| 935 | 25.0      | 1.0      | 0.0   | 0.04     | 0.25   | 0.25   | 0.04      |
